# Supplementary material for: Spinon heat transport in the three-dimensional quantum magnet PbCuTe$_2$O$_6$
Source: arXiv:2311.12221 source file (2023-11-20)
Supplement: Supplementary file 1 [file PCTO_SM.pdf]

**Supplementary Materials for:**

# Spinon heat transport in the three-dimensional quantum magnet $PbCuTe_2O_6$

## I. Sample preparation

Polycrystalline powder of $PbCuTe_2O_6$ was synthesized by a solid-state reaction of high-purity powder of PbO, CuO, and $TeO_2$. Sample P was produced from the as-grown stoichiometric polycrystalline powder, pressed and sintered in flowing argon for 12 h at 540 °C after the initial reaction. Sample P was not treated by a 5-days long annealing process which increases the grain size, thus it belongs to the small-grain polycrystal where no evident ferroelectric transition can be recognized [1]. It was cut into a rectangular bar of $3.13\times1.22\times0.2$ mm$^3$. Sample S1, with a dimension of $1.87\times0.88\times0.72$ mm$^3$, was cut from a single crystal synthesized by the top-seeded solution growth (TSSG) method. The crystal was grown using a Czochralski furnace under flowing Argon atmosphere. No inclusion of any impurity phase was detected in these TSSG-grown single crystals [2]. Sample S2, with a dimension of $3.06\times1.04\times0.75$ mm$^3$, was cut from a single crystal synthesized by the traveling solvent floating zone (TSFZ) technique. The growths were performed under flowing Argon atmospheres. It is noticed that the TSFZ-grown crystals always contain 6% $\sim$ 8% of non-magnetic impurity inclusions ($Pb_2Te_3O_8$) [1, 2]. The samples we studied are either the same (Sample S1) [3], or from the same batches (Sample S2 and Sample P) [1], of the samples used in other investigations. An exhaustive description of the growing conditions and characterizations can be found in the references [1, 2].

## II. Details of the heat transport measurements

The thermal conductivities below liquid helium temperature were measured in a dilution refrigerator, using a standard four-wire steady-state method with two $RuO_2$ chip thermometers, calibrated *in situ* against a reference $RuO_2$ thermometer. The temperature gradient

was always applied along the longest direction of the sample. One end of the sample was glued directly to the heat sink. The temperature difference between two sensors was regulated to about 5% of the average sample temperature by a heater (10 kΩ) attached to the other end of the sample (see Fig. S1).

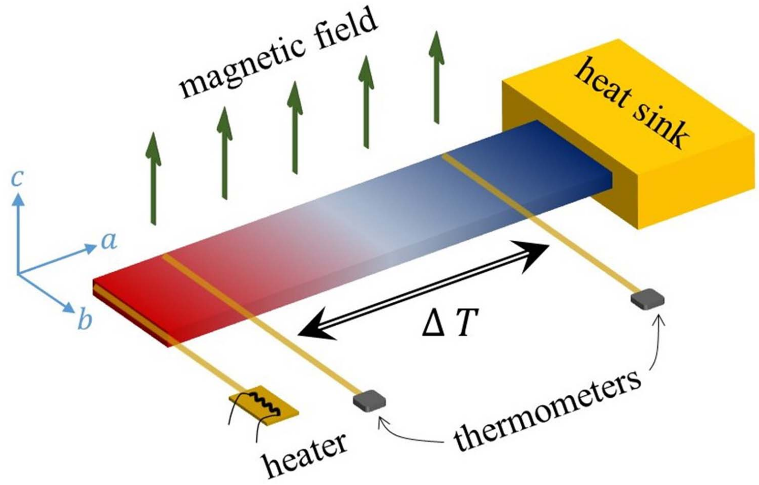


**Fig. S1:** A schematic sketch of the experimental setup. The magnetic field $H$ was applied perpendicular to the heat current.

Samples were measured in a home-built probe for higher temperature thermal conductivity data. The temperature gradient was measured by a differential AuFe/chromel-P thermocouple which had been calibrated carefully in a magnetic field.

Being an isotropic three-dimensional Heisenberg magnet, $PbCuTe_2O_6$ should not be sensitive to field direction. For consistency, magnetic field was always applied perpendicular to the heat current.

The $\kappa(H)$ isotherms have been collected in a continuous manner. For each $\kappa(H)$ isotherm, the heat sink temperature was kept at a set point, and the heater was set to a constant value that is around half of its 0 T power of the $\kappa(T)$ measurement in order to minimise the impact of $\kappa$ change on the actual sample temperature. The magnetic field was swept at a speed no more than 50 mT per minute to avoid any heating effect, in order to keep the system in a (quasi-)thermal equilibrium state. The data analysis procedure for the $\kappa(H)$ measurements is elaborated below.

## III. Data analysis of the field ramp measurements

As for the field ramp measurements, the heat sink is set at a fixed temperature. The heating power is also fixed at a certain value. So, the temperature difference between the sensors is inversely proportional to the thermal conductivity. Of course, the (average) sample temperature also changes according to the field because of the conductivity variance. In order to reduce this effect, a relatively low heating power was applied to the sample. The field effect on the sample temperatures was below 2% for all the field ramp results we present in this work.

Ruthenium oxide ($RuO_2$) is generally believed as the prime choice for thermometry at low temperature, due to its high sensitivity and low magnetic field effect [4]. However, the magnetoresistance of $RuO_2$ at dilution fridge temperatures is not negligible (see Fig. S2(b)). In the field ramp measurements, the key challenge is to properly calibrate the temperature sensors in variant fields. Below we show our approach to achieve this goal.

As a semiconductor, the $R(T)$ curves of $RuO_2$ at fixed fields roughly follows the trend of

$$R(T, H) \propto \exp\left(\frac{-\Delta}{k_B T}\right) \tag{1}$$

It is also known that the magnetoresistance of $RuO_2$ at fixed temperature is roughly linear [4]

$$R(T, H) \approx R(T, H = 0) \times (1 + \alpha H) \tag{2}$$

By combining these two relationships together, one can expect the corresponding temperature of a certain resistance value at different magnetic fields follows

$$T(R, H) = T(R, H = 0\text{ T}) + \beta \times \ln(H - \gamma) \tag{3}$$

In Fig. S2 we show one practical example step by step. The raw resistance values during one field ramp measurement is present in Fig. S2(a). At $H = 5$ T, the resistance value reads $R = 3258.47\Omega$. Taking advantage of the self-calibration matrix of sensors we got during the fixed field measurements, this resistance value is converted to a list of temperatures at different fields, as shown in Fig. S2(b). These temperatures are plotted as green squares in Fig. S2(c). They fit well into Eq. S3, as the dashed blue curve indicates. According to that, ($R = 3258.47\Omega$, $H = 5$ T) means this temperature sensor is at 628.6 mK.

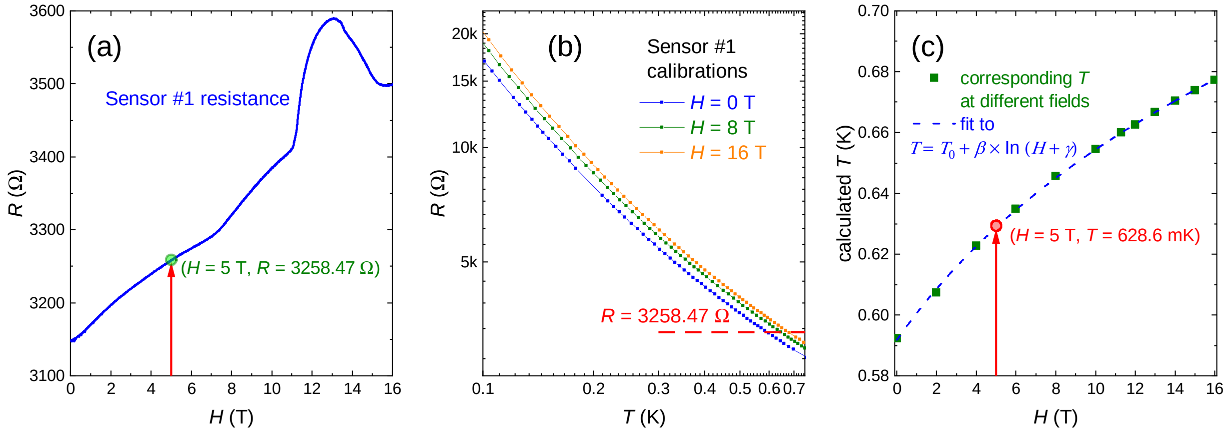


**Fig. S2:** Illustration of temperature sensor calibration in field. (a) Raw resistance data of one sensor in a field ramp measurement. The sensor reads 3258.47 Ω at $H = 5$ T. (b) Self-calibration curves of this sensor at different fields. Only three representative curves are shown for clarity. A clear magnetoresistance effect is observable. The corresponding $T$ of $R = 3258.47$ Ω at a fixed field is the crossing point of the curve with the dashed red line. (c) The corresponding $T$ of $R = 3258.47$ Ω is different at different fields. The dashed blue line is a fit to them according to Eq. S3. $T_0$ is set to $T(R = 3258.47\ \Omega, H = 0\ \text{T})$. $\beta$, and $\gamma$ are free fitting parameters.

Such procedure turns every $(R, H)$ cluster of both sensors into $T$. Based on them, the thermal conductivity and sample temperature can be calculated. The resultant $\kappa/T$ of the field ramp measurements match very well with the data extracted from the fixed field results, as evident in Fig. 1(d) of the main text. This fact rationalizes our data analysis procedure described above, and demonstrates the accuracy and reproducibility of our results.

## IV. Modeling the phonon thermal transport

The thermal conductivity curves of both single crystals at $T > 6$ K show only one peak and no distinguishable field dependence (see Fig. S3). The absence of any field dependence proves the phonon-spin scattering is not important in $PbCuTe_2O_6$, in contrast to some other spin liquid candidate materials like $\alpha{-}RuCl_3$ [5]. $PbCuTe_2O_6$ is an electrical insulator, hence the measured field-independent $\kappa$ at such temperature range is primarily phononic. The Callaway model is an established method to describe the phonon thermal conductivity [6, 7]. By applying a Debye ansatz for the phonon heat capacity, the expression for thermal

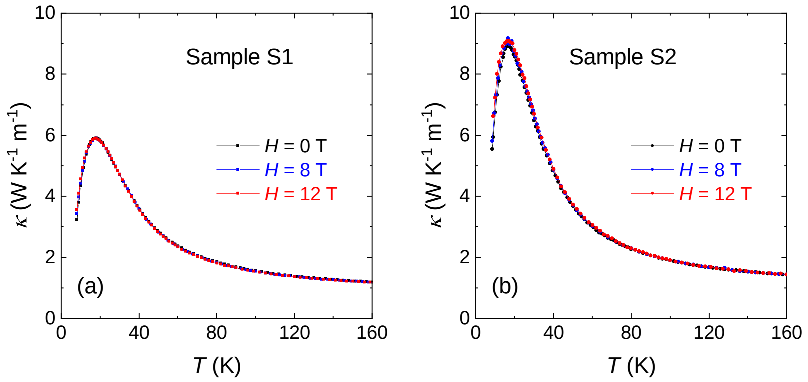


**Fig. S3:** Thermal conductivity of the two single crystals up to room temperature. $\kappa$ versus $T$ at zero and finite fields. (a) Sample S1 and (b) Sample S2.

conductivity is

$$\kappa(T) = \frac{k_B}{2\pi^2 v_s}\left(\frac{k_B T}{\hbar}\right)^3 \int_0^{\Theta_D/T} \frac{x^4 e^x}{(e^x-1)^2}\tau_c(x)\mathrm{d}x, \quad (4)$$

with frequency-dependent dimensionless energy ratio $x = \hbar\omega/k_B T$, the scattering time $\tau_c$, the sound velocity $v_s$, and the Debye temperature $\Theta_D$ ($\Theta_D = 92$ K for $PbCuTe_2O_6$ [8]). The total scattering rate is contributed by different scattering mechanisms added up according to the Matthiessen's rule: $\tau_C^{-1} = \tau_U^{-1} + \tau_D^{-1} + \tau_B^{-1}$. The contributing phonon-boundary scattering $\tau_B^{-1} = v_S/L$, the phonon-defect scattering $\tau_D^{-1} = C\omega^4$ and the phonon-phonon scattering

$$\tau_U^{-1} = BT\omega^3 \exp\left(-\frac{\Theta_D}{\alpha T}\right), \quad (5)$$

are described by empirical expressions.

We use this model to phenomenologically fit our data in the temperature range of 6 K $<$ $T <$ 100 K. The obtained parameters are shown in Table S1 and the fitting results are depicted in Fig. S4(a-c).

| Sample | $B$ [$10^{-30}$ K$^{-1}$s$^2$] | $C$ [$10^{-42}$ s$^3$] | $L$ [$10^{-6}$ m] | $\alpha$ |
|---|---|---|---|---|
| S1 | 3.56 | 2.75 | 5.49 | 2.82 |
| S2 | 3.34 | 2.12 | 9.56 | 2.42 |
| P | 3.46 | 3.25 | 5.13 | 2.72 |

**Table S1:** Obtained fitting parameters of the Callaway model for the three different samples.

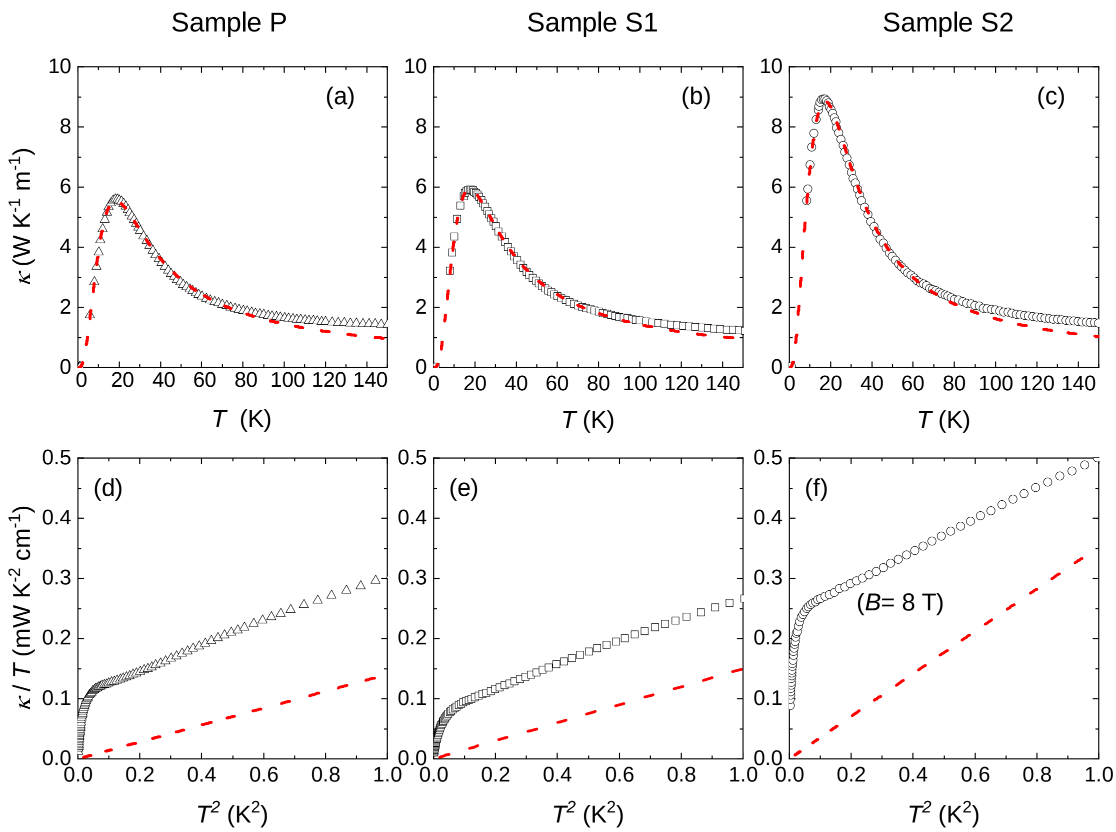


**Fig. S4:** Callaway fits to the higher-temperature thermal conductivity. Thermal conductivity $\kappa$ in zero field above 6 K for the (a) polycrystalline Sample P, the single crystals (b) Sample S1, and (c) Sample S2. The red dashed lines represent the fitting results according to the Callaway model with a fitting range up to 100 K. Comparison between the estimated phononic thermal conductivity $\kappa_{ph}$ according to the obtained parameters in Table S1 (red dashed line) and the measured low-temperature $\kappa$ data of (d) Sample P at 0 T, (e) Sample S1 at 0T, and (f) Sample S2 at 8T (due to the additional low-temperature peak without field in this sample) are presented.

By extending the phonon model with the obtained fitting parameters to low temperatures ($T < 1$ K), one can directly compare the measured data with the phenomenologically expected phonon contribution. Fig. S4(d-f) show that the predicted low-temperature phonon heat conductivity is significantly smaller than the measured $\kappa$, where is very similar to the measured data at $T^2 > 0.1$ K$^2$. In view of the fact that there is some error margin due to different geometry factors in different measurement setups, this agreement is very good. This not only corroborates our estimation of the phononic heat conductivity $\kappa_{\mathrm{ph}}$ from analyzing the $T^3$ term in the low-$T$ data (see also below). It also confirms that the peculiar temper-

ature and field dependence is not produced by a phononic scattering behavior off magnetic excitations but rather by an additional direct contribution to the heat conductivity by a magnetic transport channel.

Note that the origin of the $T^3$ dependence is rooted in the direct proportionality of $\kappa_{\rm ph}/T$ with the phononic specific heat in the low-$T$ limit. A precondition to observe it experimentally is that the phonons scatter diffusively off the crystal surfaces. A deviation from a $T^3$ behavior is usually attributed to the surface roughness of the sample that drives the sample towards the specular surface scattering limit [9]. In this context, we want to point out that some recent studies of low-temperature thermal conductivity properties of candidate quantum spin liquid materials reported field-dependent power-law behavior [10–12]. These observations of non-$T^3$ power-law $\kappa(T)$ can not be attributed only to the surface roughness since it should be field-independent. On the other hand, the fact that a moderate magnetic field can change the power-law exponent in these cases suggests the scattering of phonons is also contributed by the spin-phonon scattering. Please be aware that in our data there is no evidence for such effects which yield a deviation from $T^3$ in the heat conductivity of $PbCuTe_2O_6$.

## V. Estimation of the spinon mean free path

The dynamical properties of spinon excitations are important for understanding the QSL states. Here we provide an estimation of the mean free path $l_{\rm spinon}$ of spinons in $PbCuTeO_6$. The thermal conductivity of a mobile (quasi)particle is determined by

$$\kappa = 1/3 \times C \times v \times l, \tag{6}$$

where $C$, $v$ and $l$ are specific heat, the velocity and the mean free path of this (quasi)particle, respectively.

In the case of $PbCuTeO_6$, a linear contribution is not observed in the heat capacity measurement in the sub-Kelvin regime [2, 3]. In contrast, the dominating feature is a pronounced anomaly at about 1 K which signals the ferroelectric transition. A possible explanation is that the entropy associated with this transition obscures the magnetic specific heat but does not contribute to the heat transport because of a non-dispersive character of the dipole fluctuations. Note also that the related structural distortion is very subtle with

relative axes length changes of the order of $\sim 10^{-6}$, see Ref [13]. This provides a further explanation for the absence of any signatures of the transition in the thermal conductivity, even for measurements extending above 1 K.

In order to estimate $l_{\text{spinon}}$ we therefore rely on recent theoretical results for $C_{\text{spinon}}$ for a possible gapless QSL state in hyper-hyper-kagome systems [14], where $C_{\text{spinon}}/T \approx 2.5k_B^2/J$ per spin is estimated. By taking the $J = 1.13$ meV and structural parameters for $PbCuTeO_6$ [1], $C_{spinon}/T = 1.6$ mJ/(K$^2$mol). To evaluate $v_{\text{spinon}}$, one can also refer to the Fermi surface properties calculated within the same theoretical work [14]. By taking their results of the ground state with a spinon Fermi surface, $\epsilon_F = 0.0574J$, $k_F \sim 0.35 \times 2\pi/d$, and $e(k) = \hbar v_{\text{spinon}} k$ [14], $v_{\text{spinon}}$ is estimated to be 123 m/s. In this way, the $l_{\text{spinon}}$ of $PbCuTeO_6$ is estimated to be 133 Å(Sample S1), 434 Å(Sample S2), and 177 Å(Sample P), corresponding to 30, 99, and 41 spin spacings ($d_{S-S}$), respectively. We summarize these values in Table S2 together with results for other QSL candidate materials found in the literature.

| Material [Reference] | $l_{\text{spinon}}$ [Å] | $l_{\text{spinon}}/d_{S-S}$ |
|---|---|---|
| $PbCuTe_2O_6$ (Sample S1) [this work] | 133 | 30 |
| $PbCuTe_2O_6$ (Sample S2) [this work] | 434 | 99 |
| $PbCuTe_2O_6$ (Sample P) [this work] | 177 | 41 |
| $EtMe_3Sb[Pd(dmit)_2]_2$ [15] | $10^4$ | 1000 |
| $Cu_3V_2O_7(OH)_2 \cdot 2H_2O$ (S1) [16] | 230 | 80 |
| $Cu_3V_2O_7(OH)_2 \cdot 2H_2O$ (S2) [16] | 690 | 240 |
| $Na_2BaCo(PO_4)_2$ [17] | 36.6 | 7 |
| $1T{-}TaS_2$ [18] | $\gg 50$ | $\gg 5$ |
| $YbMgGaO4_4$ [19] | 78.4 | 23 |
| $BaCo_2(AsO_4)_2$ [12] | 123.8 | 43 |

**Table S2:** Estimation of the spinon mean free path $l_{\text{spinon}}$ of some candidate spin liquid materials, and a comparison to their corresponding spin-spin distance $d_{S-S}$.

## VI. A closer look at the thermal conductivity below $T_{\text{drop}}$

As mentioned in the main text, the depleted $\kappa_{\text{spinon}}$ signal can either indicate a spinon excitation gap, or the loss of coupling between spinons and the phonon background [20], through which $\kappa$ of an insulator is measured. We are aware that a $\mathbb{Z}_2$ QSL ground state with a gap value of $0.0259J$ was recently predicted for the $S = 1/2$ hyper-hyper-kagome QSL [14]. It matches remarkably well to our measured value for $T_{\text{drop}}$ ($\approx 0.026J_1$). However, if $T_{\text{drop}}$ indeed gauges a spinon excitation, its field dependence (see Fig. 3 of the main text) is unusual since the spin excitation gap in frustrated magnets naively should first close in field [21, 22].

If one assumes a spinon-phonon decoupling does not take any role in the temperature range covered by this study, the critical information about whether the spinon Fermi surface is fully gapped or has some "nodes" should be encoded in the details of the $\kappa_{\text{spinon}}(T)$ data below $T_{\text{drop}}$. Both power-law ($\kappa_{\text{spinon}} = b \times T^n$, corresponding to a nodal spinon Fermi surface) and exponential ($\kappa_{\text{spinon}} = A \times e^{-\Delta/k_BT}$, corresponds to fully-gapped spinon Fermi surface) fit to the representative extracted $\kappa_{spinon}(T)$ data, see Fig. S6. None of them can reproduce the data in the whole temperature range very well in their simplest form. The exponential fit yields a gap $\Delta/k_B \approx 140$ mK, i.e., a gap value which is about a factor of 2.5 smaller than the theoretically expected value [14].

On the other hand, if the $\kappa_{\text{spinon}}$ depletion results from spinon-phonon decoupling, there exists a phenomenological model that successfully described the downturn of electronic $\kappa_e/T$ in a cuprate [20]: $T_{\text{drop}} \propto a^{1/(n-1)}$, where $a$ is the $\kappa_{\text{spinon}}$ residual linear term and $n$ is a fitting parameter between 4 and 5 [20]. Since a similar consideration for spinon-phonon coupling is still missing to our knowledge, and assuming the equivalence of electron and spinon in this setting, we compare below our observations for Sample S1 and Sample P (for Sample S2, the downturn is not observed) with the predictions of this model.

In Fig. S7 the relationship of $T_{\text{drop}}$ and the residual linear term $a$ is displayed in log-log scale. According to the decoupling model [20],

$$T_{\text{drop}} = (a/Kl_s^2)^{1/(n-1)} \tag{7}$$

where $K$ is a constant which depends on the electron-phonon interaction matrix element, $l_s$ is the length of the sample along the current direction, and $n$ is a fitting parameter between 4 and 5 [20]. For a logarithmic presentation, Eq. 7 is converted into

$$\log a = (n-1)\log T_{\text{drop}} + \log(Kl_s^2), \tag{8}$$

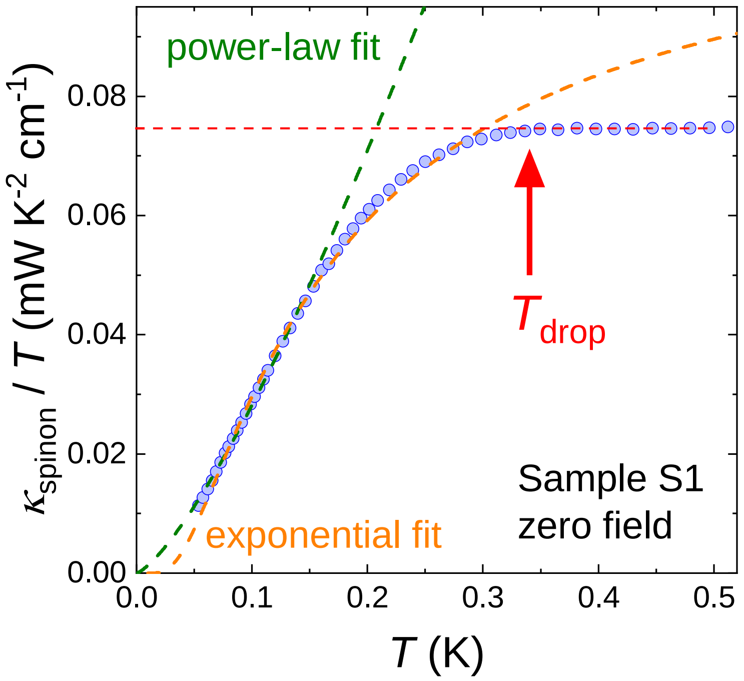


**Fig. S6:** Temperature dependence of spinon thermal conductivity in the from of $\kappa_{spinon}/T$, acquired by subtracting the phononic contribution from the total $\kappa/T$. Below a critical temperature $T_{\text{drop}} \approx 340$ mK, highlighted by the red arrow, $\kappa_{spinon}/T$ starts to drop to zero. The green and orange dashed lines are power-law and exponential fits to the data in the lowest temperature range. Data corresponds toSample S1 in zero field, see Fig. 1(a) of the main text.

where the $\log(Kl_s^2)$ term is a constant for a given sample. Especially, $K$ should not fundamentally change for a given material and $l_s$ is comparable for Sample P and Sample S1 (see Section I: Sample preparation). Hence, all the field dependent data of both samples are expected to be on the same line with a slope between $n = 4$ and $n = 5$. However, as can be seen in Fig. S7, the data do not follow such behavior, even for one given sample.

We have to mention that our analysis does not rule out the spinon-phonon decoupling as a feasible explanation for the decay of $\kappa/T$ at the low temperature limit. But a considerable modification of the original model [20] needs to be implemented in order to make it compatible with the observations.

Future work is required to clarify which of these two scenarios is valid. In any case, either of these scenarios will strongly impact the research on frustrated quantum magnets. A decoupling of phonons and spinons, if confirmed, will teach caution in the interpretation of ultra-low-temperature heat transport data. On the other hand, an experimental proof

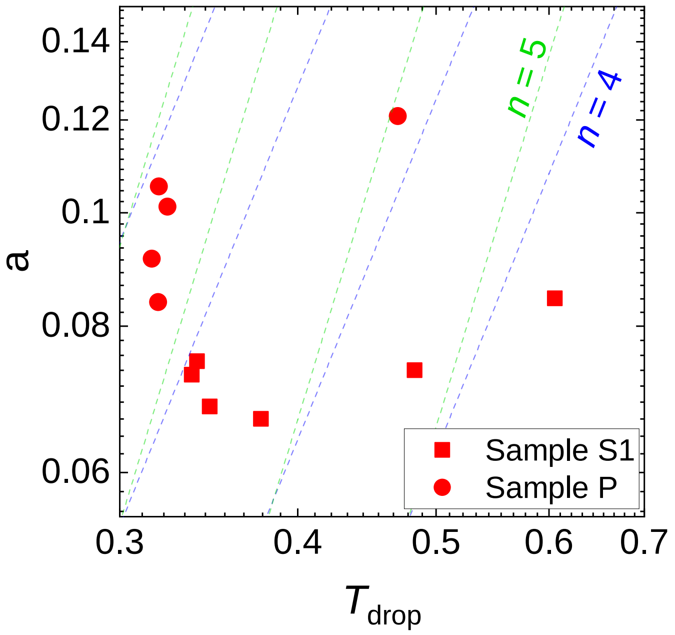


**Fig. S7:** The relationship between $a$ and $T_{\rm drop}$ of Sample S1 (square) and Sample P (circle), in logarithmic plot. The data were obtained from the results at various magnetic fields. The dashed green and blue lines are indicating the slops for $n = 5$ and $n = 4$ lines, respectively.

of a $\mathbb{Z}_2$ ground state would represent a new paradigm in quantum magnetism beyond the evidence of a spinon Fermi surface as revealed by our data for $T > T_{\rm drop}$.

## VII. Extended data shown as log-log plots and waterfall plots

In the main text, the temperature dependence of $\kappa$ was mainly plotted in the form of $\kappa/T$ aganist $T^2$ for clarify. A double-log plot of $\kappa$ against $T$ for viewing the power-law $T$ dependence of $\kappa$ in a more unbiased manner is provided by Fig. S8.

In Fig. S9 we plot a representative selection of these data. This representation reveals that the data are not compatible with a single power law. A $T^3$ behavior is only asymptotically reached at high temperature.

A different representation of the data of all samples as a function of temperature and magnetic field is shown in the waterfall plots in Fig. S10. Since our $RuO_2$ thermometers' sensitivity drops considerably with increasing temperature, the data above 1 K (and below 5 K) are regarded of lower accuracy, and thus we limited the data to $T \leq 1\ K$ in the main text. Still the data for $T > 1\ K$ yield valuable information. One can see more clearly that

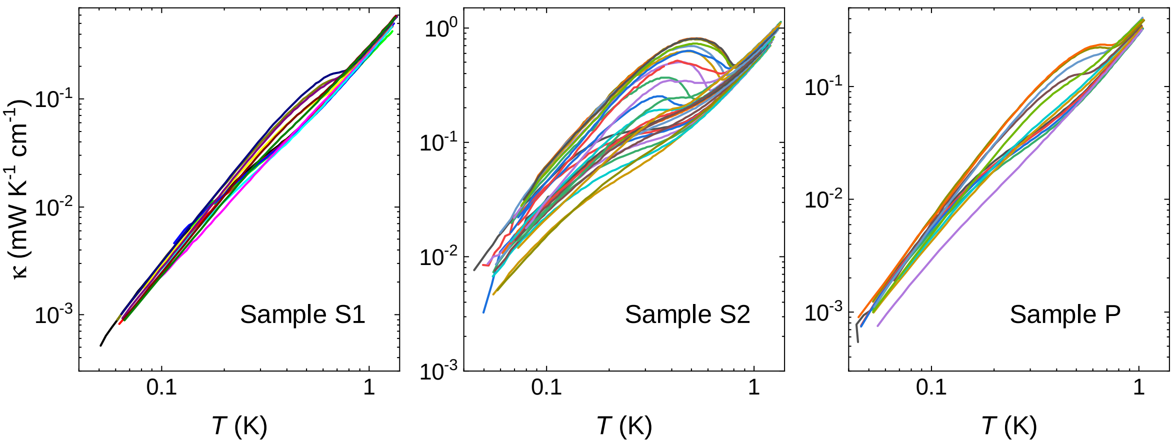


**Fig. S8:** Log-log plots of all low-temperature $\kappa(T)$ data for the three samples.

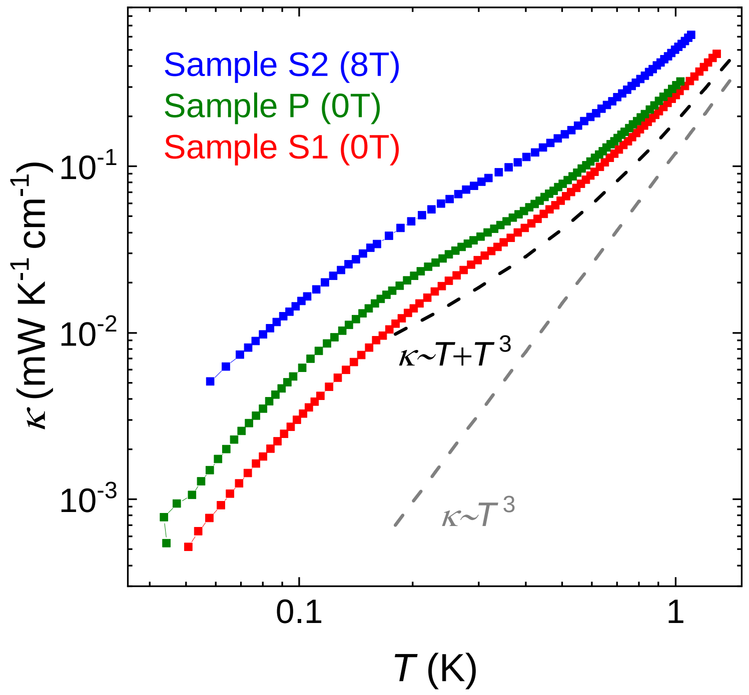


**Fig. S9:** Log-log plots of representative $\kappa(T)$ data of the three samples. Dashed lines stand for the typical $T^3$ behavior and a $T + T^3$ behavior.

the pronounced 1 K anomaly in specific heat has no observable effect in $\kappa$. Note that the related structural distortion of this 1 K ferroelectric transition is very subtle with relative axes length changes of the order of $\sim 10^{-6}$, see Ref [13]. This provides a explanation for the absence of any signatures of the transition in the thermal conductivity.

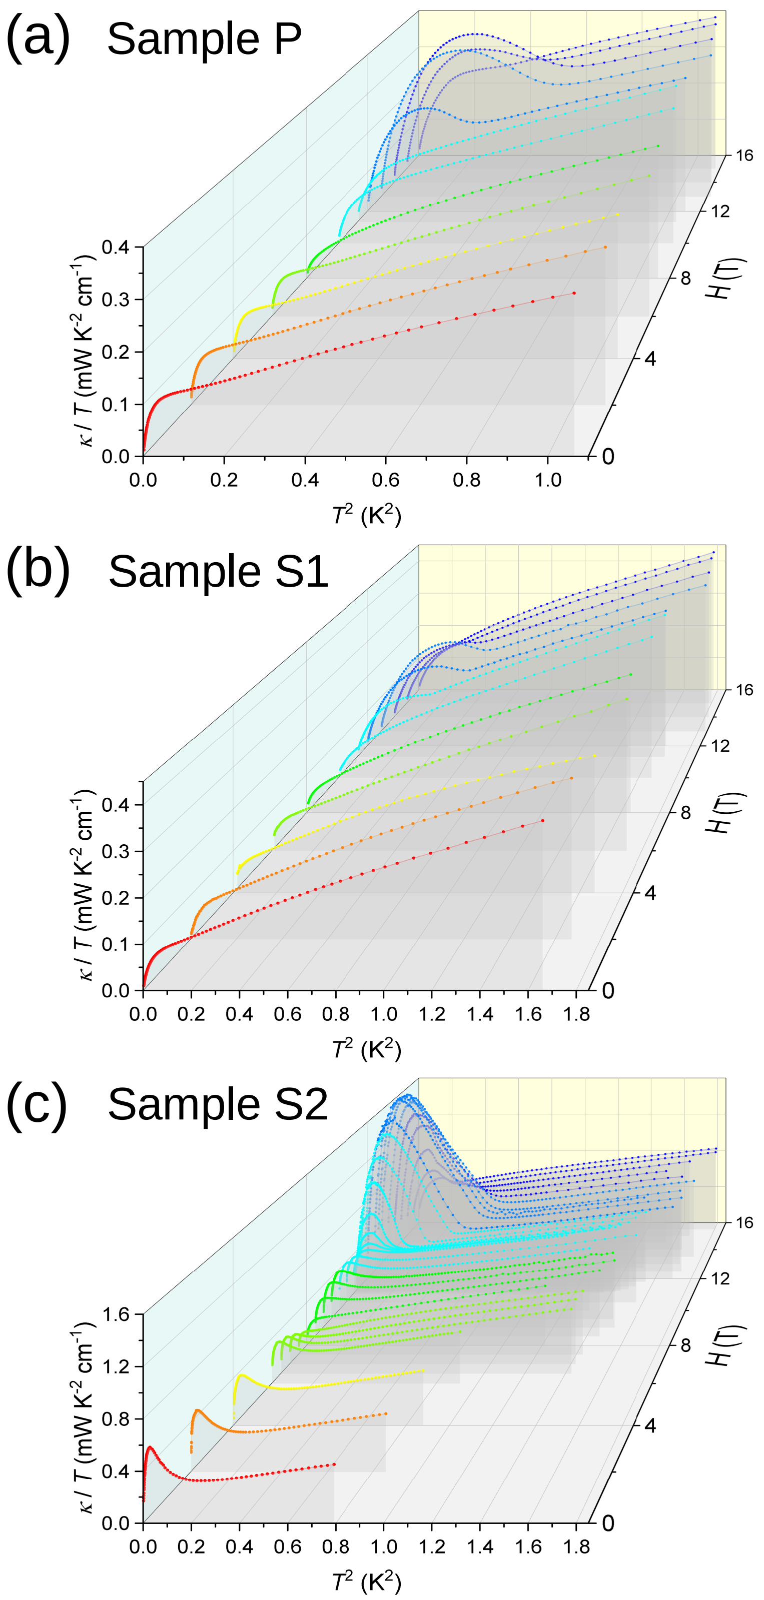


**Fig. S10:** Waterfall plots of the low-temperature thermal conductivity of (a) Sample P, (b) Sample S1, and (c) Sample S2.

## VIII. More discussion on the additional lower-temperature $\kappa/T(T)$ peak

Despite the fact that magnetic order could not be detected below 11 T in previous works on $PbCuTe_2O_6$ samples [1–3, 8, 13, 23], we tend to attribute this feature to a magnetic order induced by inclusions. This is reasonable since muon spin relaxation and nuclear magnetic resonance data reveal a slowing down of spin fluctuations which imply the proximity of the system to magnetic order [23]. The critical nature is further confirmed by a diverging Grüneisen parameter [13]. Considering the non-magnetic $Pb_2Te_3O_8$ second phase inclusions of Sample S2 [2], one may therefore conjecture that weak sample-dependent magnetic order can be induced, if the fine balance between magnetic interactions is disturbed by strain fields around the inclusions of the second phase. Apparently, this specialty of Sample S2 together with the symmetry reduction connected with the structural phase transition and the ferroelectric order seems sufficient to tip the system towards magnetic order.

[1] S. Chillal et al., *Evidence for a three-dimensional quantum spin liquid in* $PbCuTe_2O_6$, Nat. Commun. **11**, 2348 (2020).

[2] A.R.N. Hanna et al., *Crystal growth, characterization, and phase transition of* $PbCuTe_2O_6$, Phys. Rev. Materials **5**, 113401 (2021).

[3] P. Eibisch et al., *Field-induced effects in the spin liquid candidate* $PbCuTe_2O_6$, Phys. Rev. B **107**, 235133 (2023).

[4] G. G. Ihas, L. Frederick, and J. P. McFarland, *Low Temperature Thermometry in High Magnetic Fields*, J. Low Temp. Phys. **113** 963–968 (1998).

[5] R. Hentrich et al., *Unusual Phonon Heat Transport in* $\alpha$-$RuCl_3$: *Strong Spin-Phonon Scattering and Field-Induced Spin Gap*, Phys. Rev. Lett. **120**, 117204 (2018).

[6] J. Callaway, *Low-Temperature Lattice Thermal Conductivity*, Phys. Rev. **122**, 787 (1961).

[7] J. Callaway, *Model for Lattice Thermal Conductivity at Low Temperatures*, Phys. Rev. **113**, 1046 (1959).

[8] B. Koteswararao et al., *Magnetic properties and heat capacity of the three-dimensional frustrated* $S = 1/2$ *antiferromagnet* $PbCuTe_2O_6$, Phys. Rev. B **90**, 035141 (2014).

[9] S. Y. Li et al., *Low-temperature phonon thermal conductivity of single-crystalline* $Nd_2CuO_4$: *Effects of sample size and surface roughness*, Phys. Rev. B **77**, 134501 (2008).

[10] Q. Barthelemy et al., *Heat conduction in herbertsmithite: Field dependence at the onset of the quantum spin liquid regime*, Phys. Rev. B **107**, 054434 (2023).

[11] X. C. Hong et al., *Phonon thermal transport shaped by strong spin-phonon scattering in a Kitaev material* $Na_2Co_2TeO_6$, on-line preprint at arXiv:2306.16963

[12] C. P. Tu et al., *Evidence for gapless quantum spin liquid in a honeycomb lattice*, on-line preprint at arXiv:2212.07322

[13] C. Thurn et al., *Spin liquid and ferroelectricity close to a quantum critical point in* $PbCuTe_2O_6$, npj Quantum Mater. **6**, 95 (2021).

[14] L. E. Chern and Y. B. Kim, *Theoretical study of quantum spin liquids in* $S = 1/2$ *hyper-hyperkagome magnets: Classification, heat capacity, and dynamical spin structure factor*, Phys. Rev. B **104**, 094413 (2021).

[15] M. Yamashita et al., *Highly mobile gapless excitations in a two-dimensional candidate quantum*

*spin liquid*, Science **328**, 1246 (2010).

[16] D. Watanabe et al., *Emergence of nontrivial magnetic excitations in a spin-liquid state of kagome volborthite*, Proc. Natl. Acad. Sci. U.S.A. **113**, 8653-8657 (2016).

[17] N. Li et al., *Possible itinerant excitations and quantum spin state transitions in the effective spin-1/2 triangular-lattice antiferromagnet* $Na_2BaCo(PO_4)_2$, Nat. Commun. **11**, 4216 (2020).

[18] H. Murayama et al., *Effect of quenched disorder on the quantum spin liquid state of the triangular-lattice antiferromagnet* $1T-TaS_2$, Phys. Rev. Research **2**, 013099 (2020).

[19] X. Rao et al., *Survival of itinerant excitations and quantum spin state transitions in* $YbMgGaO_4$ with chemical disorder, Nat. Commun. **12**, 4949 (2021).

[20] M. F. Smith et al., *Origin of anomalous low-temperature downturns in the thermal conductivity of cuprates*, Phys. Rev. B **71**, 014506 (2005).

[21] X. C. Hong et al., *Heat transport of the kagome Heisenberg quantum spin liquid candidate* $YCu_3(OH)_{6.5}Br_{2.5}$: *Localized magnetic excitations and a putative spin gap*, Phys. Rev. B **106**, L220406 (2022).

[22] M. Fu et al., *Evidence for a Gapped Spin-Liquid Ground State in a Kagome Heisenberg Antiferromagnet*, Science **350**, 655-658 (2015).

[23] P. Khuntia et al., *Spin liquid state in the 3D frustrated antiferromagnet* $PbCuTe_2O_6$: *NMR and Muon spin relaxation studies*, Phys. Rev. Lett. **116**, 107203 (2016).
